# Supplementary material for: Uni-MoE: Scaling Unified Multimodal LLMs with Mixture of Experts
Source: arXiv:2405.11273 source file (2024-05-18)
Supplement: Supplementary file 1 [file additional_tables.tex]

\begin{table*}[t]

\centering
\caption{\label{more-experts-und}
\textbf{Ablation Study of Uni-MoE performances with more image-text training data and experts}. For models with \textit{X}B, \textit{X} refers to the size of the language model.  For our models with \textit{Y}E, \textit{Y} refers to the number of experts.  
Names are abbreviated due to space limits. I: Image; T: Text; A: Audio; S: Speech; V: Video; AOK: A-OKVQA \cite{aokvqa}; OK: OK-VQA~\cite{okvqa}; MMB: MMBench~\cite{mmbench}; POPE~\cite{li-etal-2023-evaluating}; VQA$^T$: TextVQA~\cite{singh2019towards}; SEED:SEED-Bench~\cite{seedBENCH}; MMVet~\cite{yu2023mm}.
``EHSL'' refers to the English High School Listening Test we collected, containing long/short speech types.
$^\ddagger$ indicates that this model employs enormous or unknown data during training.
Uni-MoE still achieves better comprehensive performances, demonstrating the mixed training data management capacities of MoE.}
\resizebox{1.0\linewidth}{!}{
\begin{tabular}{l|cccccccc|ccc}
\hline
\textbf{Method} & \textbf{AOK} & \textbf{OK} & \textbf{VQAv2} & \textbf{MMB} & \textbf{POPE} &\textbf{VQA$^T$} & \textbf{SEED} & \textbf{MMVet} & \textbf{RACE-Audio} & \textbf{EHSL} & \textbf{ActivityNet-QA} \\
\hline
\textit{Any-Modality Understanding} & & & & & & & & &\\
Macaw-LLM~\cite{lyu2023macaw}  & 1.90\% & 5.70\% & 20.73\% & 3.84\% & - & - & - & - & 4.04\%/3.00\% & 0.67\%/2.00\% &  -\\
X-InstructBLIP~\cite{panagopoulou2023x} & 21.52\% & 30.61\% & 37.77\% & 8.96\% & - & - & - & - & 16.33\%/18.88\% & 0.67\%/2.00\% &-\\
\hline
\textit{Dense Model} & & & & & & & & & \\
AnyMAL-70B (I,T,A,V)~\cite{moon2023anymal} & -&42.6\% &64.2\% & -& -& 32.9\% & -&-&-&-&-\\
IDEFICS-80B (I,T)~\cite{laurenccon2024obelics} & - & -& 60.0\% & 54.5\% & - & 30.9\% & -& - & - & - &- \\
LLaVA-1.5-7B (I,T)~\cite{liu2023improved} & 70.92\% & 55.09\% & 75.9\% & 72.7\% & 85.9\% & 58.2\% & -& 30.5\% & -& - & -  \\
LLaVA-1.5-13B (I,T)~\cite{liu2023improved} & 73.54\% & 61.93\% & 78.9\% & 73.4\% & 85.9\% & 60.2\% & - & 35.4\% & -& - & - \\
BLIP-2(FlanT5-xxl)-11B (I,T)~\cite{li2023blip2} & 39.06\% & 53.7\% & 65.0\% & - & 85.3\% & 42.8\% & -&-&-&-&-\\
InstructBLIP(Vicuna)-13B (I,T)~\cite{dai2024instructblip} & 58.30\% & 41.02\% & - & - & 50.7\% &- &25.6\% & - & -& - & -\\
Shikra-13B (I,T)~\cite{chen2023shikra} &- & -& 77.4\% & 58.8\% & - & -&-& - & -& - & -\\
LLaMA-VID-13B (I,T,V)~\cite{li2023llamavid} & -& -& 80.0\%& 66.6\% & 86.0\% & 49.0\% & 62.3\% &- &-&-& 47.5\% \\
MiniGPT-4-7B (I,T)~\cite{zhu2023minigpt} & 36.06\% & 29.31\% & - & 23.0\% & -& - & 42.84\% & 22.1\% & -& - & - \\
LLaMA-Adapter-v2-7B (I,T)~\cite{gao2023llama} &-&-&-&39.5\% & -&-&-&31.4\% &-&-&-\\
Qwen-VL-7B$^\ddagger$ (I,T)~\cite{qwen} & - & 58.6\% & 78.8\% & 68.2\% & - & 63.8\% & 56.3\% & - & -& - & - \\
MobileVLM-3B (I,T)~\cite{chu2023mobilevlm} & - & - & - & 59.6\% & 84.9\% & 47.5\% & - & - & - & - & -\\
LLaVA-Phi-3B (I,T)~\cite{zhu2024llava_phi} & -& -& 71.4\% & 59.8\% & 85.0\% & 48.6\% & -&28.9\% & - & - & - \\
{Single-Modality-Expert-Task2} (I,T) & 67.07\% & 62.91\% & 75.18\% & 71.26\% & 84.7\% & 45.16\%& 60.63\%& 27.8\% &-&-&- \\
{Single-Modality-Expert-Task5} (I,T,S) & 58.86\% & 56.01\% & 67.35\% & 65.80\% &62.48\% &43.78\% &53.50\%  &26.9\% &  30.78\%/24.90\% & 9.33\%/12.00\% & -\\
{Single-Modality-Expert-Task6} (I,T,S) & 58.69\% & 57.77\% & 68.74\% & 67.53\%  &65.84\% &44.24\% &55.21\% &25.6\%  &32.59\%/29.02\% & 18.67\%/8.00\%&-\\
%{Single-Modality-Expert-Task2} & 21.21\% & 32.20\% & 33.26\% & 65.36\%  \\
%{Single-Modality-Expert-Task5} & 14.45\% & 22.68\% & 26.71\% & 62.03\%  \\
%{Single-Modality-Expert-Task6} & 15.69\% & 24.36\% & 26.77\% & 61.05\%  \\
\hline
Sparse Model  & & & & & & & & & \\
MoE-Lla\\

%{Uni-MoE w/ MoE-Task1 1 epoch} & 19.01\% & 30.12\% & 31.05\% & 56.84\%  \\
%{Uni-MoE w/ MoE-Task1 2 epoch} & 19.16\% & 26.84\% & 29.97\% & 56.84\%  \\
%{Uni-MoE w/ MoE-Task1 3 epoch} & 17.48\% & 25.46\% & 28.50\% & 55.43\%  \\ 
%{Uni-MoE w/ MoE-Task1-short 1 epoch} & 22.11\% & 33.12\% & 32.49\% & 54.54\% \\
%{Uni-MoE w/ MoE-Task1-short 2 epoch} & 22.97\% & \textbf{36.18}\% & 33.36\% & 63.06\% \\
%{Uni-MoE w/ MoE-Task1-short 3 epoch} & \textbf{25.14\%} & 34.64\% & 35.17\% & 62.37\% \\

%{Uni-MoE w/ MoE-Task1 1 epoch} & 62.88\% & 57.77\% & 69.82\% & 68.84\%  \\
{Uni-MoE w/ MoE-Task1 (4E)} (I,T,S) & 61.22\% & 57.63\% & 68.42\% & 68.15\% &56.67\% & 39.12\% & 52.58\% &30.1\% & 47.08\%/47.08\% & 41.33\%/36.00\% & - \\
%{Uni-MoE w/ MoE-Task1 3 epoch} & 59.91\% & 57.07\% & 68.05\% & 67.28\%  \\ 
%{Uni-MoE w/ MoE-Task2 1 epoch} & 66.20\% & 63.02\% & 74.41\% & 71.17\%  \\
{Uni-MoE w/ MoE-Task2 (4E)} (I,T,S,V)& 65.07\% & 62.10\% & 73.87\% & 70.50\% & 85.43\% &41.56\% &60.54\% &28.2\% & 49.65\% /49.37\% & 42.00\%/48.00\% & 42.2\% \\
%{Uni-MoE w/ MoE-Task3 1 epoch} & 65.07\% & 61.38\% & 73.66\% & 69.52\%  \\
{Uni-MoE w/ MoE-Task3 (4E)} (I,T,A,V) & 64.28\% & 61.96\% & 73.87\% & 69.82\% & 86.10\% & 40.63\% &59.16\% &31.7\% & - & 42.8\% \\
%{Uni-MoE w/ MoE-Task2 1 epoch} & 22.93\% & 32.98\% & 35.80\% & 60.54\%  \\
%{Uni-MoE w/ MoE-Task2 2 epoch} & 24.14\% & 34.72\% & 37.98\% & 59.79\%  \\
%{Uni-MoE w/ MoE-Task3 1 epoch} & 23.43\% & 35.06\% & \textbf{38.54}\% & 67.12\%  \\
%{Uni-MoE w/ MoE-Task3 2 epoch} & 22.76\% & 35.18\% & 37.51\% & \textbf{67.47}\%  \\
{Uni-MoE w/ MoE-Task4 (4E)} (I,T,S,V) & 69.08\% & 66.02\% & 76.4\% & 73.3\% & 86.0\% & 49.2\% & 63.4\% & 32.6\% & 64.21\%/64.72\% & 48.00\%/58.67\% & 45.6\%\\
+ Aux\_loss & 69.61\% & 66.13\%& 76.0\%& 72.6\%&  84.8\%  & 48.2\% & 63.3\% & 31.7\% & 63.86\%/64.24\%& 50.00\%/54.00\% & 45.2\%\\
{Uni-MoE w/ MoE-Task4 (8E)} (I,T,S,V) \\
+ Aux\_loss \\
\hline
\end{tabular}}

\end{table*}

\begin{table}[t]

\centering
\caption{\label{image-text-und}
\textbf{Model performance on image-text understanding and reasoning benchmarks}. Uni-MoE still achieves better performance compared to models with the single expert configuration.}
\resizebox{1.0\linewidth}{!}{
\begin{tabular}{l|cccc}
\hline
\textbf{Method} & \textbf{A-OKVQA} & \textbf{OK-VQA} & \textbf{VQAv2} & \textbf{MMBench} \\
\hline
Macaw-LLM~\cite{lyu2023macaw}  & 1.90\% & 5.70\% & 20.73\% & 3.84\%  \\
X-InstructBLIP~\cite{panagopoulou2023x} & 21.52\% & 30.61\% & 37.77\% & 8.96\% \\
\hline
{Single-Modality-Expert-Task2} & 67.07\% & 62.91\% & 75.18\% & 71.26\%  \\
{Single-Modality-Expert-Task5} & 58.86\% & 56.01\% & 67.35\% & 65.80\%  \\
{Single-Modality-Expert-Task6} & 58.69\% & 57.77\% & 68.74\% & 67.53\%  \\
%{Single-Modality-Expert-Task2} & 21.21\% & 32.20\% & 33.26\% & 65.36\%  \\
%{Single-Modality-Expert-Task5} & 14.45\% & 22.68\% & 26.71\% & 62.03\%  \\
%{Single-Modality-Expert-Task6} & 15.69\% & 24.36\% & 26.77\% & 61.05\%  \\
\hline
%{Uni-MoE w/ MoE-Task1 1 epoch} & 19.01\% & 30.12\% & 31.05\% & 56.84\%  \\
%{Uni-MoE w/ MoE-Task1 2 epoch} & 19.16\% & 26.84\% & 29.97\% & 56.84\%  \\
%{Uni-MoE w/ MoE-Task1 3 epoch} & 17.48\% & 25.46\% & 28.50\% & 55.43\%  \\ 
%{Uni-MoE w/ MoE-Task1-short 1 epoch} & 22.11\% & 33.12\% & 32.49\% & 54.54\% \\
%{Uni-MoE w/ MoE-Task1-short 2 epoch} & 22.97\% & \textbf{36.18}\% & 33.36\% & 63.06\% \\
%{Uni-MoE w/ MoE-Task1-short 3 epoch} & \textbf{25.14\%} & 34.64\% & 35.17\% & 62.37\% \\

{Uni-MoE w/ MoE-Task1 1 epoch} & 62.88\% & 57.77\% & 69.82\% & 68.84\%  \\
{Uni-MoE w/ MoE-Task1 2 epoch} & 61.22\% & 57.63\% & 68.42\% & 68.15\%  \\
{Uni-MoE w/ MoE-Task1 3 epoch} & 59.91\% & 57.07\% & 68.05\% & 67.28\%  \\ 
{Uni-MoE w/ MoE-Task2 1 epoch} & 66.20\% & 63.02\% & 74.41\% & 71.17\%  \\
{Uni-MoE w/ MoE-Task2 2 epoch} & 65.07\% & 62.10\% & 73.87\% & 70.50\%  \\
{Uni-MoE w/ MoE-Task3 1 epoch} & 65.07\% & 61.38\% & 73.66\% & 69.52\%  \\
{Uni-MoE w/ MoE-Task3 2 epoch} & 64.28\% & 61.96\% & 73.87\% & 69.82\%  \\
%{Uni-MoE w/ MoE-Task2 1 epoch} & 22.93\% & 32.98\% & 35.80\% & 60.54\%  \\
%{Uni-MoE w/ MoE-Task2 2 epoch} & 24.14\% & 34.72\% & 37.98\% & 59.79\%  \\
%{Uni-MoE w/ MoE-Task3 1 epoch} & 23.43\% & 35.06\% & \textbf{38.54}\% & 67.12\%  \\
%{Uni-MoE w/ MoE-Task3 2 epoch} & 22.76\% & 35.18\% & 37.51\% & \textbf{67.47}\%  \\
\hline
\end{tabular}}

\end{table}

\begin{table}[t]
\centering

\caption{\label{hign_school}
 \textbf{Zero-shot Results on our collected English High School Listening Test (Long Speech)}. It aims to assess the long/short speech understanding abilities of MLLMs in real-world applications of speech recognition.}
\resizebox{0.90\linewidth}{!}{
\begin{tabular}{l|cc}
\hline
\textbf{Method} & \textbf{Long} & \textbf{Short}\\
\hline
{Macaw-LLM~\cite{lyu2023macaw}}&0.67\%&2.00\%\\
X-InstructBLIP~\cite{panagopoulou2023x} & 0.67\% & 2.00\% \\
\hline
Single-Modality-Expert-Task4 & 12.67\% & 6.00\% \\
Single-Modality-Expert-Task5 & 9.33\% & 12.00\% \\
{Single-Modality-Expert-Task6} & 18.67\% & 8.00\% \\
{Single-Modality-Expert-Task7} & 34.67\% & 46.00\% \\
\hline
%{Uni-MoE w/ MoE-Task1 1 epoch} & 32.67\% & 38.00\% \\
{Uni-MoE w/ MoE-Task1 2 epoch} & 41.33\% & 36.00\% \\
%{Uni-MoE w/ MoE-Task2 1 epoch} & \textbf{43.33\%} & 36.00\% \\
{Uni-MoE w/ MoE-Task2 2 epoch} & \textbf{42.00\%} & \textbf{48.00\%} \\
\hline
\end{tabular}}

\end{table}
